# Supplementary material for: MoVE-KD: Knowledge Distillation for VLMs with Mixture of Visual Encoders
Source: arXiv:2501.01709 source file (2025-03-18)
Supplement: Supplementary file 1 [file X_suppl.tex]

\clearpage
\setcounter{page}{1}
\maketitlesupplementary
\appendix
\setcounter{table}{0}
\setcounter{figure}{0}

\begin{figure}[!h]
    \centering
    \includegraphics[width=0.9\linewidth]{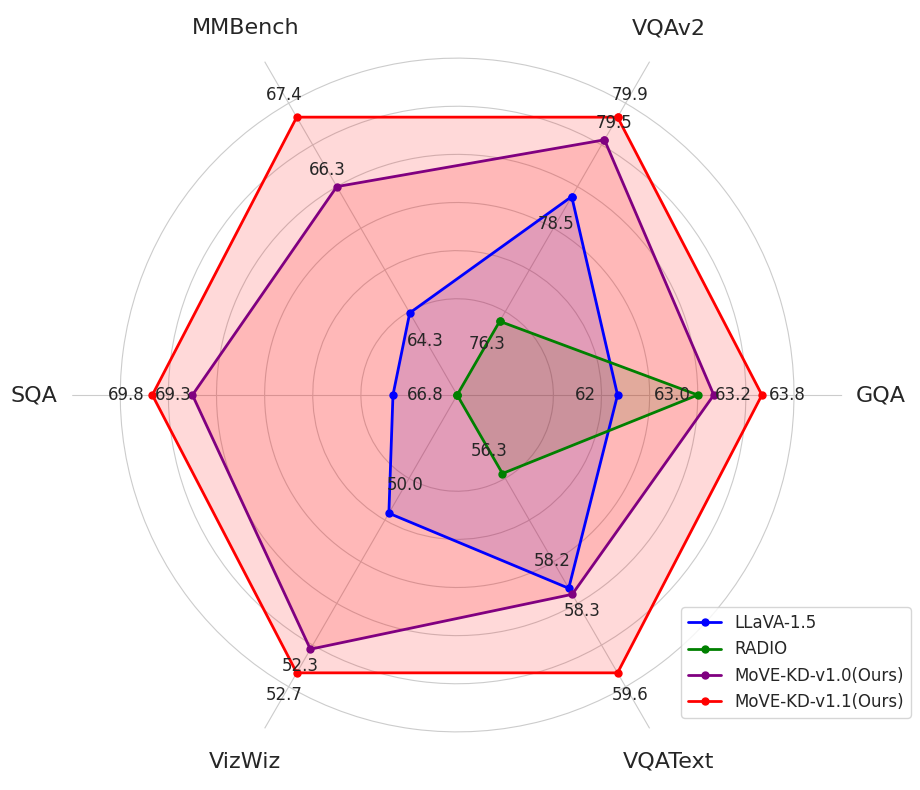}
    \caption{Comparison of MoVE-KD-v1.0 and MoVE-KD-v1.1.}
    \label{fig:radar}
\end{figure}

\section{Overview}

In the appendix, we present more implementation details, additional experiments and visualization. For further insights, please refer to the anonymous website at \url{https://MoVE-KD.github.io/} to watch the video explanation, and the full code will be published in the future.

\begin{figure*}[t] % 使用 figure* 环境使图片占据全栏
  \centering
  \begin{subfigure}{0.49\textwidth} % 保持子图比例
    \centering 
    \includegraphics[width=1.0\linewidth]{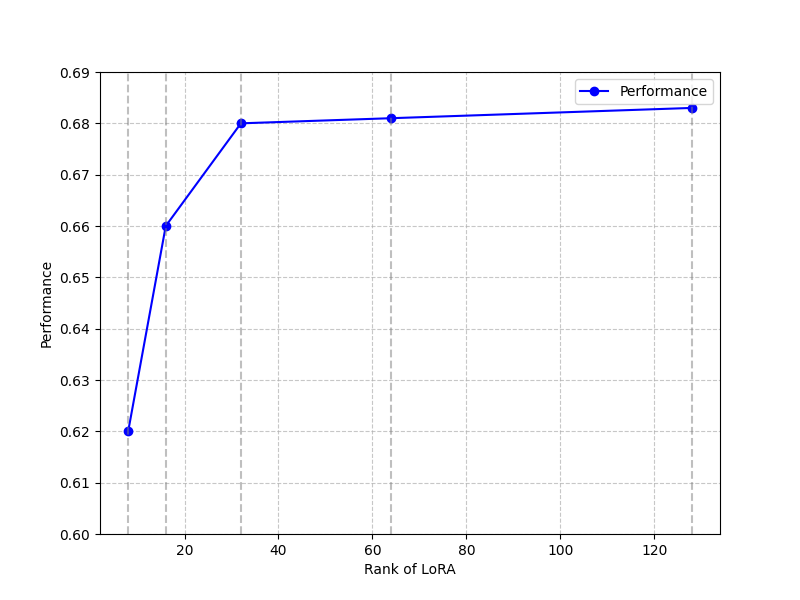}
    \caption{Impact of the rank of LoRA}
    \label{fig:rank}
  \end{subfigure}
  \hfill
  \begin{subfigure}{0.49\textwidth}
    \centering 
    \includegraphics[width=1.0\linewidth]{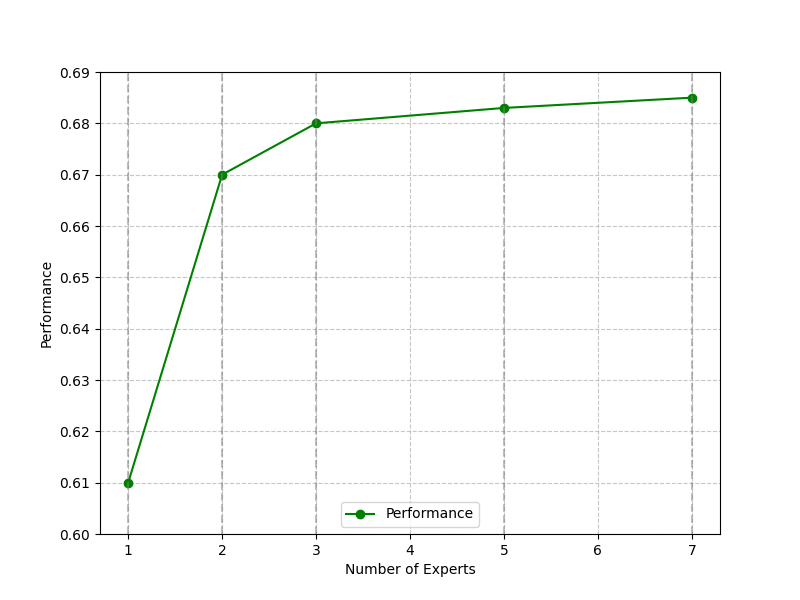}
    \caption{Impact of number of experts}
    \label{fig:experts}
  \end{subfigure}
  \caption{The impact of the rank of LoRA and the number of experts on MoLE performance. Marginal benefits diminish when the LoRA rank exceeds 32 or the number of experts is greater than 3.}
  \label{fig:mole}
\end{figure*}

\section{Implementation Details}

\subsection{Dataset}

We train the student model followed by the official dataset in LLaVA-1.5 \cite{liu2023improvedllava} and LLaVA-NeXT \cite{liu2024llavanext}, including VQA~\cite{goyal2017making,hudson2019gqa,mao2016generation,schwenk2022okvqa}, OCR~\cite{mishra2019ocr,sidorov2020textcaps}, region VQA~\cite{kazemzadeh2014referitgame,mao2016generation,krishna2017visual}, visual conversation~\cite{liu2024visual} and language conversation~\cite{sharegpt}.
% We adopt multiple strategies to reduce training costs and enhance efficiency, detailed as follows:
% \begin{enumerate}
%     \item For all VQA datasets, QA pairs from the same training image are merged into a single conversation.
%     \item For ShareGPT~\cite{sharegpt}, we filter out invalid conversations as \cite{touvron2023llama}. Unlike Vicuna~\cite{touvron2023llama}, long conversations that surpass 2048 tokens are truncated rather than splitting into multiple conversations. This results in $\sim$40K conversations.
%     \item Each QA pair in A-OKVQA~\cite{schwenk2022okvqa} is augmented $k$ times, where $k$ is the number of choices per question, to counterbalance the lack of multiple-choice data.
%     \item 80K conversations are sampled from OCRVQA \cite{mishra2019ocr}.
%     \item For Visual Genome, we sample 10 annotations for images with additional annotations.
%     \item For RefCOCO, conversations are dissected into segments, each containing fewer than 10 conversations.
%     \item We obverse that language conversations are often longer than visual ones. For each batch, we sample conversations only from a single modality, and this speeds up the training by 25\%, and does not affect the outcome.
% \end{enumerate}

\subsection{Benchmarks}

We conduct comprehensive experiments on several widely used visual understanding benchmarks, followed by a list.

\textbf{VQA-v2.}~\citep{goyal2017making} The VQA-v2 benchmark evaluates the model’s visual perception capabilities through open-ended questions. It consists of 265,016 images, covering various real-world scenes and objects, providing rich visual contexts for the questions. For each question, there are 10 ground truth answers provided by human annotators, which allows for a comprehensive evaluation of the performance of different models in answering the questions accurately.

\textbf{GQA.}~\citep{hudson2019gqa} The GQA benchmark comprises three parts: scene graphs, questions, and images. The image part contains images, the spatial features of images, and the features of all objects in images. The questions in GQA are designed to test the understanding of visual scenes and the ability to reason about different aspects of an image.

\textbf{TextVQA.}~\citep{singh2019towards} The TextVQA benchmark focuses on the comprehensive integration of diverse text information within images. It meticulously evaluates the model’s text understanding and reasoning abilities through a series of visual question-answering tasks with rich textual information. Models need to not only understand the visual content of the images but also be able to read and reason about the text within the images to answer the questions accurately.

\textbf{VizWiz.}~\citep{gurari2018vizwiz} The VizWiz dataset originates from a natural visual question-answering setting where blind people each took an image and recorded a spoken question, together with 10 crowd-sourced answers per visual question. The benchmark evaluates models to recognize, read, and reason about the visual elements and textual information in the images. This dual requirement challenges models to demonstrate robust text comprehension and logical reasoning skills, ensuring they can effectively integrate diverse information sources to provide accurate answers.

\textbf{POPE.}~\citep{li2023evaluating} The POPE benchmark is primarily used to evaluate the degree of Object Hallucination in models. It reformulates hallucination evaluation by requiring the model to answer a series of specific binary questions regarding the presence of objects in images. Accuracy, Recall, Precision, and F1 Score are effectively employed as reliable evaluation metrics to precisely measure the model's hallucination level under three different sampling strategies.

\textbf{ScienceQA.}~\citep{lu2022learn} The ScienceQA benchmark covers diverse domains, including natural science, language science, and social science. Within each subject, questions are categorized first by the topic, then by the category, and finally by the skill. This hierarchical categorization results in 26 topics, 127 categories, and 379 skills, providing a comprehensive and diverse range of scientific questions. It provides a comprehensive evaluation of a model's capabilities in multimodal understanding, multi-step reasoning, and interoperability.

\textbf{MME.}~\citep{fu2023mme} The MME benchmark is also a comprehensive benchmark meticulously designed to thoroughly evaluate various aspects of a model's performance. It consists of 14 sub-tasks that specifically aim to evaluate both the model's perceptual and cognitive abilities. By utilizing manually constructed instruction-answer pairs and concise instruction design, it effectively mitigates issues such as data leakage and unfair evaluation of model performance.

\textbf{MMBench.}~\citep{liu2023mmbench} The MMBench benchmark comprehensively evaluates the model's overall performance across multiple dimensions by incorporating multiple-choice questions. It includes three levels of ability dimensions. The first level (L1) consists of two main abilities, perception and reasoning. The second level (L2) expands based on the first level, including six sub-abilities. The third level (L3) further refines the second level, encompassing 20 specific ability dimensions. This hierarchical structure enables a comprehensive evaluation of the model's various capabilities.

\subsection{Configurations}
\begin{itemize}
\item \textbf{Input resolution:}
    \begin{itemize}
    \item \textbf{CLIP:} $336 \times 336$
    \item \textbf{EVA:} $1024 \times 1024$
    \item \textbf{ConvNeXt:} $1024 \times 1024$
    \item \textbf{SAM:} $1024 \times 1024$
    \end{itemize}
\item \textbf{Checkpoints:}
    \begin{itemize}
    \item \textbf{CLIP:} \href{https://huggingface.co/openai/clip-vit-large-patch14-336}{clip-vit-large-patch14-336}
    \item \textbf{EVA:} \href{https://huggingface.co/Yuxin-CV/EVA-02/blob/main/eva02/det/eva02_L_coco_det_sys_o365.pth}{eva02\_L\_coco\_det\_sys\_o365.pth}
    \item \textbf{ConvNeXt:} \href{https://huggingface.co/laion/CLIP-convnext_xxlarge-laion2B-s34B-b82K-augreg-soup}{CLIP-convnext\_xxlarge-laion2B-s34B-b82K-augreg-soup}
    \item \textbf{SAM:} \href{https://huggingface.co/facebook/sam-vit-large}{sam-vit-large}
    \end{itemize}
\item \textbf{MoLE:}
    \begin{itemize}
    \item \textbf{Number of experts:} 3
    \item \textbf{Rank of LoRA:} 32
    \end{itemize}
\end{itemize}

\definecolor{mygray}{gray}{.92}
\definecolor{ForestGreen}{RGB}{34,139,34}
\definecolor{Forestred}{RGB}{220,50,50}
\definecolor{goldenrod}{RGB}{250, 250, 235}
\newcolumntype{a}{>{\columncolor{goldenrod}}c}
\begin{table*}[!h]
    \centering
    % \hspace{2mm}
    \setlength{\tabcolsep}{2.8pt}
    
    \footnotesize
	\centering
	
    \begin{tabular}{p{3cm} c | p{1cm}<{\centering} p{1cm}<{\centering} p{1cm}<{\centering} p{1cm}<{\centering} p{1cm}<{\centering} p{1cm}<{\centering} p{1cm}<{\centering} p{1cm}<{\centering}}
        \shline
        \textbf{Method} & \textbf{LLM} &\textbf{VQA}$^{\text{V2}}$ & \textbf{GQA} &  \textbf{VQA}$^{\text{Text}}$ & \textbf{VizWiz} & \textbf{POPE} & \textbf{SQA}& \textbf{MME} & \textbf{MMB} \\
        \hline
        \rowcolor{mygray}
        \multicolumn{10}{c}{\textit{1.7B Models}} \\
        LLaVA-1.5 \cite{liu2023improvedllava} & MobileLLaMA-1.4B \cite{chu2023mobilevlm}  & 71.5 & 55.4 & 42.6 & 28.6 & 84.3 & 56.0 & 1145.7 & 47.0 \\
        + MSE & MobileLLaMA-1.4B \cite{chu2023mobilevlm}  & 72.0 & 55.8 & 42.5 & 29.3 & 84.2 & 55.4 & 1161.8 & 47.1 \\
        \rowcolor{goldenrod}
        + MoVE-KD \texttt{\scriptsize{(Ours)}} & MobileLLaMA-1.4B \cite{chu2023mobilevlm}  & \textbf{72.9} & \textbf{56.6} & \textbf{43.4} & \textbf{32.1} & \textbf{84.8} & \textbf{56.1} & \textbf{1182.3} & \textbf{47.4}\\
        \hline
        
        \rowcolor{mygray}
        \multicolumn{10}{c}{\textit{7B Models}} \\
        InstructBLIP \cite{liu2024visual} & Vicuna-7B \cite{zheng2023judging} & - & 49.2 & 50.1 & 34.5 & - & 60.5 & - & 36 \\
        Qwen-VL \cite{bai2023qwen} & Qwen-7B \cite{bai2023qwen} & 78.8 & 59.3 & 63.8 & 35.2 & - & 67.1 & 1487.5 & 38.2\\
        \hline
        LLaVA-1.5 \cite{liu2023improvedllava} & Vicuna-7B \cite{zheng2023judging} & 78.5 & 62.0 & 58.2 & 50.0 & 85.9 & 66.8 & 1510.7 & 64.3 \\
        + MSE & Vicuna-7B \cite{zheng2023judging} & 79.0 & 62.4 & 56.7 & 50.9 & 84.7 & 67.6 & 1507.6 & 62.9 \\
        + RADIO \cite{ranzinger2024radio} & Vicuna-7B \cite{zheng2023judging} & 76.3 & 63.0 & 56.3 & - & 86.2 & - & - & - \\
        \rowcolor{goldenrod}
        + MoVE-KD \texttt{\scriptsize{(Ours)}} & Vicuna-7B \cite{zheng2023judging} & \textbf{79.5} & \textbf{63.2} & \textbf{58.3} & \textbf{52.3} & \textbf{86.9} & \textbf{69.3} & \textbf{1524.5} & \textbf{66.3} \\
        \hline
        LLaVA-NeXT \cite{liu2024llavanext} & Vicuna-7B \cite{zheng2023judging} & 81.8 & 64.2 & 64.9 & 57.6 & 86.5 & 70.1 & 1519.0 & 67.4 \\
        + MSE & Vicuna-7B \cite{zheng2023judging} & 82.0 & 63.5 & 63.1 & 57.2 & 86.4 & 70.3 & 1526.9 & 67.0 \\
        \rowcolor{goldenrod}
        + MoVE-KD \texttt{\scriptsize{(Ours)}} & Vicuna-7B \cite{zheng2023judging} & \textbf{82.3} & \textbf{64.5} & 63.7 & \textbf{58.0} & \textbf{86.7} & \textbf{70.7} & \textbf{1537.2} & \textbf{67.6} \\
        \hline

        \rowcolor{mygray}
        \multicolumn{10}{c}{\textit{13B Models}} \\
        InstructBLIP \cite{liu2024visual} & Vicuna-13B \cite{zheng2023judging} & - & 49.5 & 50.7 & 33.4 & 78.9 & 63.1 & 1212.8 & - \\
        \hline
        LLaVA-1.5 \cite{liu2023improvedllava} & Vicuna-13B \cite{zheng2023judging} & 80.0 & 63.3 & 61.3 & 53.6 & 85.9 & 71.6 & 1531.3 & 67.7 \\
        \rowcolor{goldenrod}
        + MSE & Vicuna-13B \cite{zheng2023judging} & 80.1 & 63.7 & 58.4 & 54.6 & 84.7 & 71.9 & 1543.3 & 68.8 \\
        + MoVE-KD \texttt{\scriptsize{(Ours)}} & Vicuna-13B \cite{zheng2023judging} & \textbf{80.6} & \textbf{64.2} & 59.7 & \textbf{55.7} & 85.7 & \textbf{73.2} & \textbf{1568.1} & \textbf{70.2} \\
        \hline
        LLaVA-NeXT \cite{liu2024llavanext} & Vicuna-13B \cite{zheng2023judging} & 82.8 & 65.4 & 67.1 & 60.5 & 86.2 & 73.6 & 1575.0 & 70 \\
        + MSE & Vicuna-13B \cite{zheng2023judging} & 82.4 & 65.1 & 64.5 & 60.7 & 86.3 & 73.4 & 1568.4 & 70.3 \\
        \rowcolor{goldenrod}
        + MoVE-KD \texttt{\scriptsize{(Ours)}} & Vicuna-13B \cite{zheng2023judging} & \textbf{83.1} & \textbf{65.7} & 65.8 & \textbf{60.9} & \textbf{86.8}  & \textbf{73.7} & \textbf{1579.3} & \textbf{70.6}  \\

        \shline
	\end{tabular}
     \vspace{-2mm}
     \caption{\textbf{Performance of MoVE-KD and other methods} (inlcude MSE KD.) }
    \vspace{-2mm}
	\label{tab:X_mse}
\end{table*}

\section{Additional experiments}
\subsection{Comparison of MSE-based distillation 
} In the ablation study, we demonstrate the gap between the distillation method based on simple interpolation with mean squared error (MSE) loss and MoVE-KD. Due to space constraints in the main text, we present this method (referred to as MSE) as a baseline in Tab. \ref{tab:X_mse} to highlight the superiority and effectiveness of our proposed improvements.

\subsection{Settings of MoLE
} We further investigated the impact of the rank of LoRA and the number of experts in MoLE on the experimental results, using the average performance across various benchmarks (excluding MME \cite{fu2023mme}) as the evaluation metric. As shown in Fig. \ref{fig:mole}, when the rank of LoRA exceeds 32 and the number of experts exceeds 3, the marginal benefits diminish. Therefore, to balance performance and computational cost, we choose the most appropriate hyperparameter settings.

\begin{figure*}[!h]
    \centering
    \includegraphics[width=0.95\linewidth]{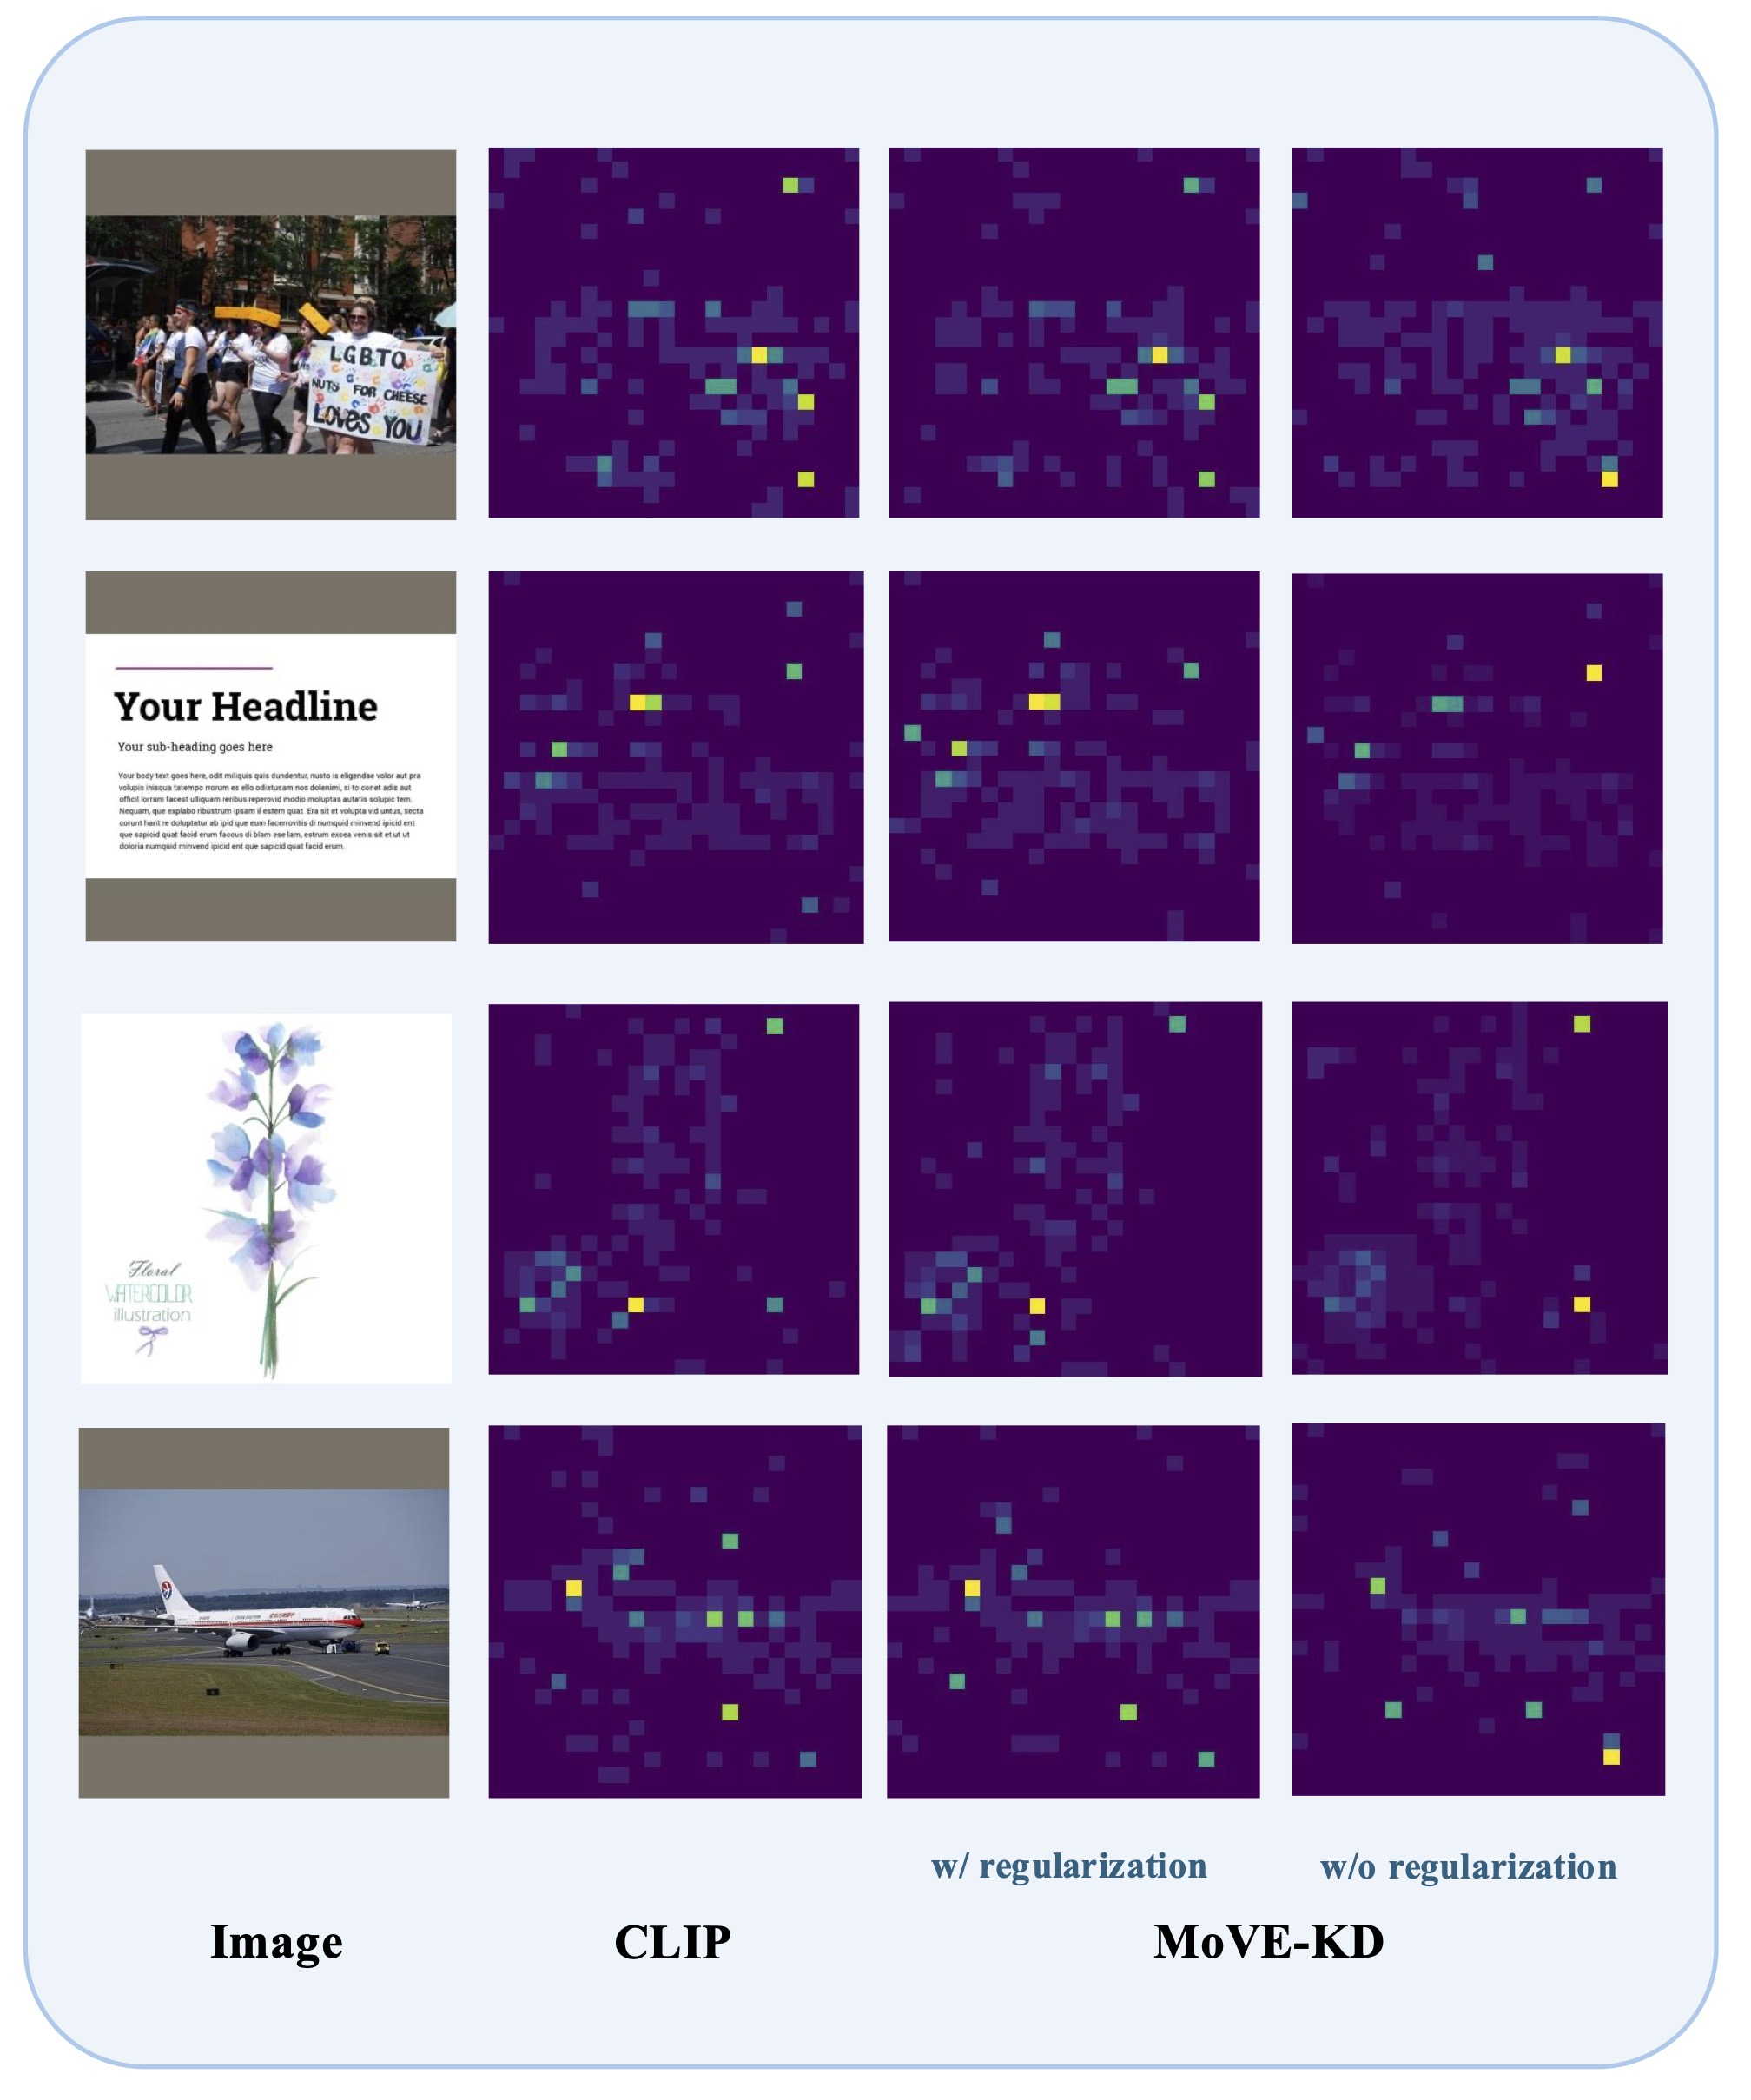}    
    \caption{\textbf{The visualization of the  [\texttt{CLS}] attention of CLIP and MoVE-KD (w/ and w/o regularization).} }
    \label{fig:attntion_suppl}
\end{figure*}

\section{Visualization}
In Fig. \ref{fig:attntion_suppl}, we additionally show the results without [\texttt{CLS}] attention regularization, which shows that the [\texttt{CLS}] attention has a low correlation with key information.
